# Supplementary material for: Networks with many structural scales: a Renormalization Group perspective
Source: arXiv:2406.19104 source file (2024-12-16)
Supplement: Supplementary file 1 [file 1-SupInf.pdf]

# Supplemental Material: Networks with many structural scales: a Renormalization Group perspective

Anna Poggialini,[1,2] Pablo Villegas,[2,3,*] Miguel A. Muñoz,[4,3] and Andrea Gabrielli[2,5]

[1]*Dipartimento di Fisica Università "Sapienza", P.le A. Moro, 5, I-00185 Rome, Italy.*
[2]*'Enrico Fermi' Research Center (CREF), Via Panisperna 89A, 00184 - Rome, Italy*
[3]*Instituto Carlos I de Física Teórica y Computacional, Universidad de Granada, E-18071, Granada, Spain.*
[4]*Departamento de Electromagnetismo y Física de la Materia, Universidad de Granada, Granada 18071, Spain*
[5]*Dipartimento di Ingegneria Civile, Informatica e delle Tecnologie Aeronautiche, Università degli Studi "Roma Tre", Via Vito Volterra 62, 00146 - Rome, Italy.*

## CONTENTS

1. Asymptotic limit of $\lambda_F$ 2
2. Asymptotically scale-invariant graphs 3
3. Regular lattices 3
4. Scale-dependent networks 4
5. Bethe lattices 5
6. Barabási-Albert networks 6
7. $(u, v)-$flowers 7
8. Kim and Holme networks 9
9. Dyson network 10
10. HMN networks 11
11. Human Connectome network 13
References 14

* pablo.villegas@cref.it

## 1. ASYMPTOTIC LIMIT OF $\lambda_F$

Let us assume to have a scale-invariant network for which $\omega(\lambda) = A\lambda^\gamma$, with $\gamma = d_s/2 - 1$ and that $\lambda_{max}$ do not depend on $N$ (reasonable if the maximum node degree does not scale with $N$) [1]. Since the total number of eigenvalues is $N$, i.e. the number of network nodes, we have

$$A \int_0^{\lambda_{max}} d\lambda\, \lambda^\gamma \equiv A \frac{\lambda_{max}^{\gamma+1}}{\gamma+1} = N \,,$$

which implies $A = \frac{\gamma+1}{\lambda_{max}^{\gamma+1}} N$. On the other hand, by the definition of the Fiedler eigenvalue $\lambda_F$, we need to have [2],

$$A \int_0^{\lambda_F} d\lambda\, \lambda^\gamma = 1 \,,$$

from which we can derive the scaling relation $\lambda_F \sim N^{-2/d_s}$.

Under these hypotheses, the specific heat can be written as

$$C(t) = t^2 \left( \left\langle \lambda^2 \right\rangle_t - \left\langle \lambda \right\rangle_t^2 \right) = t^2 \frac{\left( A \int_0^{\lambda_{max}} d\lambda\, \lambda^\gamma e^{-\lambda t} \right) \left( A \int_{\lambda_F}^{\lambda_{max}} d\lambda\, \lambda^{\gamma+2} e^{-\lambda t} \right) - \left( A \int_{\lambda_F}^{\lambda_{max}} d\lambda\, \lambda^{\gamma+1} e^{-\lambda t} \right)^2}{\left( A \int_0^{\lambda_{max}} d\lambda\, \lambda^\gamma e^{-\lambda t} \right)^2} \,, \tag{1}$$

where the lower integration extreme for the integrals of the first and second moments of $\lambda$ with time dependent measure $\hat{\rho}(t)$ is explicitly limited to $\lambda_F$ as the fundamental eigenvalue $\lambda = 0$ does not contribute and in this way we can explicitly study the effect of the $N$-dependent gap $\lambda_F \sim N^{-2/d_s}$ for finite $N$.

By the change of integration variable $u = \lambda t$, we can write

$$C(t) = \frac{\left( \int_0^{u_{max}} du\, u^\gamma e^{-u} \right) \left( \int_{\lambda_F t}^{u_{max}} du\, u^{\gamma+2} e^{-u} \right) - \left( \int_{\lambda_F t}^{u_{max}} du\, u^{\gamma+1} e^{-u} \right)^2}{\left( \int_0^{u_{max}} du\, u^\gamma e^{-u} \right)^2} \tag{2}$$

with $u_{max} = \lambda_{max} t$.

Let us now evaluate $C(t_F)$ with $t_F = \alpha/\lambda_F \sim N^{2/d_s}$ where $C(t)$ is expected to deviate from the constant value $d_s/2$ because of finite size effects giving a constant gap. In this case, due to the exponential factor in the integrals, we can take with no danger $u_{max} \to +\infty$. Consequently, we can write

$$C(\alpha/\lambda_F) = \frac{\Gamma(\gamma+1) \int_\alpha^\infty du\, u^{\gamma+2} e^{-u} - \left( \int_\alpha^\infty du\, u^{\gamma+1} e^{-u} \right)^2}{\Gamma^2(\gamma+1)} = \frac{\Gamma(\gamma+1)\Gamma(\gamma+3,\alpha) - \Gamma^2(\gamma+2,\alpha)}{\Gamma^2(\gamma+1)} \,, \tag{3}$$

where $\Gamma(x)$ is the complete Euler Gamma function and $\Gamma(x,\alpha) = \int_\alpha^\infty du\, u^{x-1} e^{-u}$ is the lower incomplete Euler Gamma function. Equation (3) immediately shows that for different $N$ we get the same large time value for the specific heat $C(t)$, different from the infinite $N$ value $d_s/2$, at corresponding times $t = \alpha/\lambda_F$ where $\lambda_F \sim N^{-2/d_s}$, while this value depends on $\alpha$. In particular, by using the large $\alpha$ asymptotic expansion of $\Gamma(x,\alpha)$ in Eq. (3) we get that the main $\alpha$ dependence characterized by the following exponential decay:

$$C(\alpha/\lambda_F) = \frac{\alpha^{\gamma+2} e^{-\alpha}}{\Gamma(\gamma+1)} \,. \tag{4}$$

Finally, it is simple to note that in the limit $\alpha \to 0^+$ Eq. (3) correctly coincides with the limit $N \to \infty$ of Eq. (2) at finite $t$:

$$C(t) = \frac{\Gamma(\gamma+1)\Gamma(\gamma+3) - [\Gamma(\gamma+2)]^2}{[\Gamma(\gamma+1)]^2} = \gamma + 1 = d_s/2 \,,$$

which explains the plateau value.

## 2. ASYMPTOTICALLY SCALE-INVARIANT GRAPHS

Despite its simplicity, the request for a unique power-law behavior to hold on to all the support of the spectrum may seem too severe to be easily detected in both synthetic and real graphs. However, a large set of networks satisfies a much weaker but equally relevant condition: $\omega(\lambda) \sim \lambda^{\gamma}$ in the limit $\lambda \to 0$. Networks that meet this asymptotic condition are scale-invariant graphs. The results shown in the main text can be derived, in a more general way, for the asymptotic case using the Tauberian and Abelian theorems [3]. In particular, one can write

$$C(t)log(N) = -t^2 \frac{d}{dt} h(t). \tag{5}$$

If $\omega(\lambda) \sim \lambda^{\gamma}$ in for $\lambda \to 0$, then $h(t) \sim t^{-1}$ in the limit $t \to \infty$ and $C(t)log(N) \sim \gamma + 1 < \infty$ in the same regime. In this context, the study of the spectral dimension $d_s$ fits the well-known asymptotic definitions $d_{\mathrm{s}} = -2 \lim_{t\to\infty} \frac{\ln p_t(G,v)}{\ln t}$ and $\lim_{\lambda_N \to 0} \omega_N(\lambda_N)$ when these limits exist for infinite-sized graphs and where $p_t(G, v)$ is the return probability of a random walk to a generic vertex $v$ at time $t$ and $\omega_N(\lambda_N)$ is the spectral density of normalized Laplacian operator.

## 3. REGULAR LATTICES

For consistency and to avoid spurious results, we first study the most straightforward trivial scale-invariant structures: regular lattices. As shown in Figure 1, the $\tau$ peak at short diffusion times reflects the characteristic resolution scale of the system (or, in other words, the 'cutoff' scale, $\Lambda$). We have analyzed different simple cases (both in 2D and 3D) to check the correspondence between the specific heat and the expected dimension of the network, using both $\hat{L}$ and $\hat{L}_{RW}$. We emphasize that, in this particular case, both Laplacians are formally equivalent, as for regular lattices, $P(\kappa) = \delta(\kappa - \kappa_0)$, where $k_0$ represents the coordination number of the homogeneous structure.

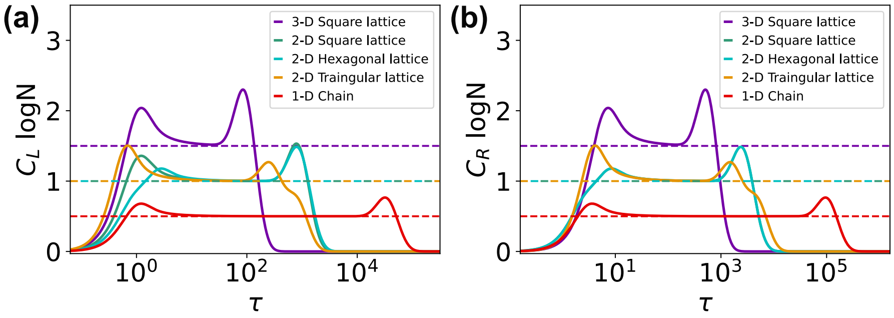


FIG. 1. **Regular lattices.** Specific heat versus diffusion time by using (a) $\hat{L}$ and (b) $\hat{L}_{RW}$. All networks show a plateau for the expected dimension of any lattice for both cases.

## 4. SCALE-DEPENDENT NETWORKS

We have conducted extensive simulations to analyze the specific heat of Erdös-Rényi networks of different mean connectivity. Figure 2 shows the expected specific heat versus the diffusion time for different sizes of the system, which shows that there is no scaling for large networks. Note also that $C_L$ presents a single peak, pointing to a scale that corresponds to the system size.

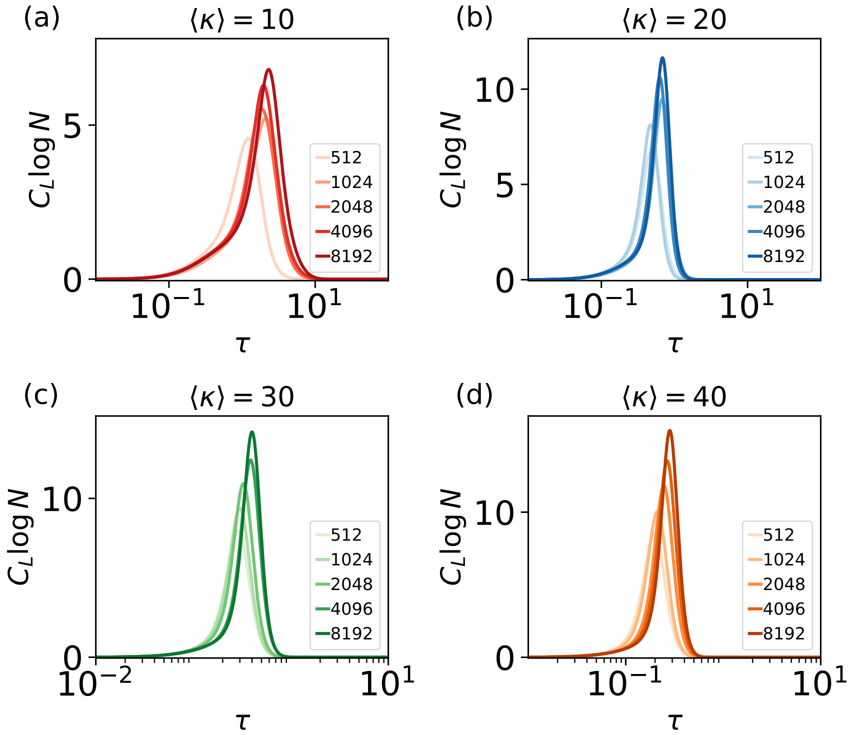


FIG. 2. **Erdös-Rényi networks.** Specific heat versus diffusion time for different network sizes (see legend) and mean connectivity: (a) $\langle\kappa\rangle = 10$, (b) $\langle\kappa\rangle = 20$, (c) $\langle\kappa\rangle = 30$, (d) $\langle\kappa\rangle = 40$. All curves have been averaged over $10^2$ network realizations.

## 5. BETHE LATTICES

One of the paradigmatic cases of self-similar networks is those of Bethe lattices with coordination number $z > 2$. Figure 3 shows the specific heat for different Bethe lattices with coordination numbers $z = 3, 4, 5$ and 6. Note that the specific heat monotonically grows for all networks at short times. Still, the heat capacity asymptotically converges to a constant value with a spectral dimension $d_S = 2$ (see Figure 3). The scaling of the Fielder eigenvalue confirms such a constant value (see also the theoretical proof below), as reported in Figure 4.

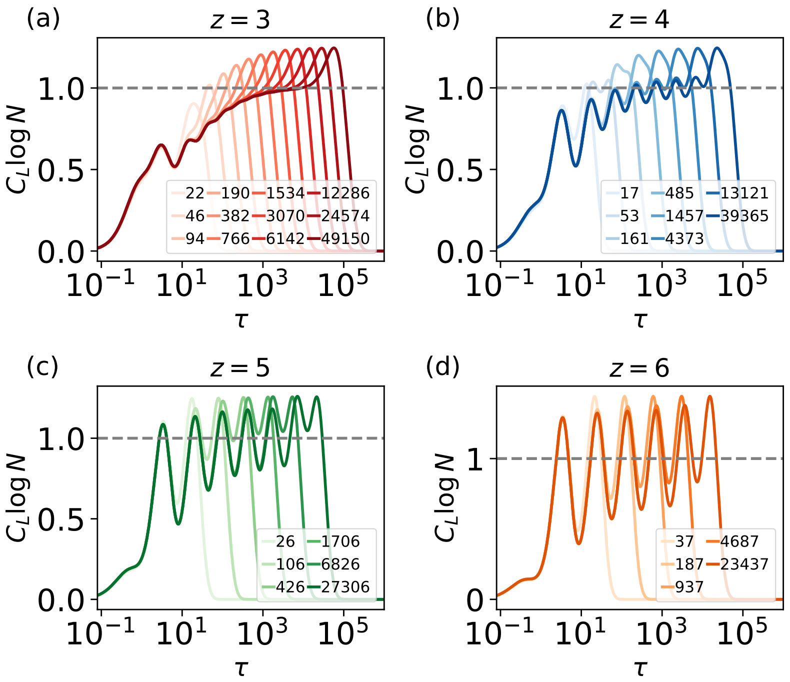


FIG. 3. **Bethe lattice.** Specific heat versus system size for Bethe lattices of different coordination numbers: (a) $z = 3$, (b) $z = 4$, (c) $z = 5$, (d) $z = 6$. The dashed gray line shows the value associated with the scaling of the Fiedler eigenvalue in Figure 4.

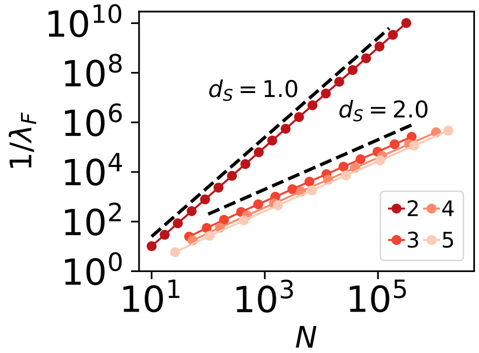


FIG. 4. **Fiedler scaling.** Scaling of the inverse of the Fiedler eigenvalue versus system size for different Bethe lattices and different values of $z$ (see legend). Black dashed lines correspond to $1/\lambda_F \sim N^{2/d_S}$. Bethe lattices with $z \geq 3$ present generic scaling with associated spectral dimension $d_S = 2$.

We now rigorously demonstrate that all Bethe lattices exhibit an identical spectral dimension $d_S = 2$. For convenience, let us consider a regular Cayley tree where all nodes present a branching ratio $b$ and $r$ iterations. The total number of nodes is

$$N_r = \frac{b^r - 1}{b - 1} \Rightarrow r = \frac{\log(Nb - N + 1)}{\log b}$$

Following the results of Erzan and Tuncer [4], we know that,

$$\lambda_F \sim (b-1)\, b^{-r} = \frac{b-1}{b^{\frac{\log(Nb-N+1)}{\log b}}}$$

and thus,

$$\frac{1}{\lambda_F} \sim \frac{b^{\frac{\log(Nb-N+1)}{\log b}}}{b-1}$$

where the upper term simply involves the change of base formula $\log_b a = \frac{\log_c a}{\log_c b}$. Finally,

$$\frac{1}{\lambda_F} \sim N + \frac{1}{b-1}$$

By comparison with the scaling form for $1/\lambda_F$, $d_S = 2$, regardless of the value of $b$.

## 6. BARABÁSI-ALBERT NETWORKS

We have analyzed BA networks with subsequent values of $m > 1$ for both cases $\hat{L}$ and $\hat{L}_{RW}$. As shown in Figures 5 and 6, BA networks show no sign of scaling properties for $m > 1$, nor in the specific heat, where any plateau is present, nor in the analysis of the Fiedler eigenvalue, where only the network with $m = 1$ presents a bona-fide scaling with $d_S = 2$.

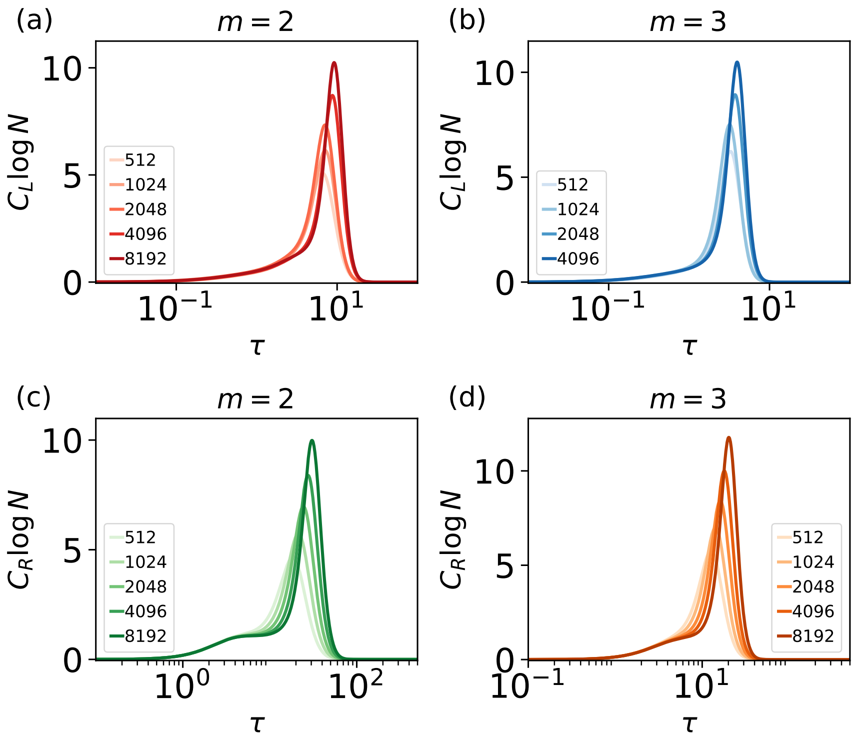


FIG. 5. **Barabási-Albert.** Specific heat versus system size for BA networks of different $m$ for: (a) $\hat{L}$, $m = 2$, (b) $\hat{L}$, $m = 3$, (c) $\hat{L}_{RW}$, $m = 2$, and (d) $\hat{L}_{RW}$, $m = 3$. All cases show no plateau, evidencing the absence of scale-invariant properties of the networks.

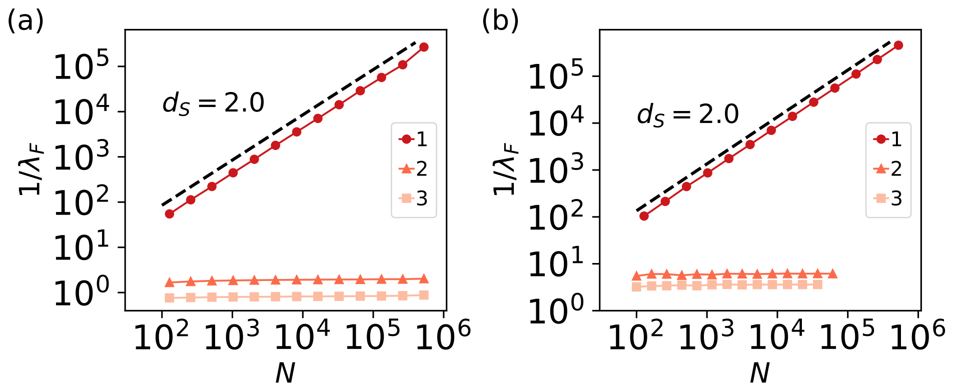


FIG. 6. **Spectral dimension.** Scaling of the inverse of the Fiedler eigenvalue versus system size for different Barabási-Albert networks and different values of $m$ (see legend) by using (a) the Laplacian $\hat{L}$ and (b) the normalized Laplacian $L_{RW}$. In both cases, only the case with $m = 1$ is truly scale-invariant with spectral dimension $d_S = 2$.

## 7. $(u, v)-$FLOWERS

The *(u, v)-flowers* are deterministic and recursive graphs [5]. Let us briefly describe how such networks are built: At step $t = 0$, the graph $G(0)$ corresponds to a dimer, that is, two nodes connected by a link. The structure of successive $G(t > 0)$ is driven by both the parameters $u$ and $v$, together with $1 \leq u \leq v$. $G(t)$ is built by replacing each link of $G(t-1)$ with two parallel links of, respectively, length $u$ and $v$, as shown in Fig. 7.

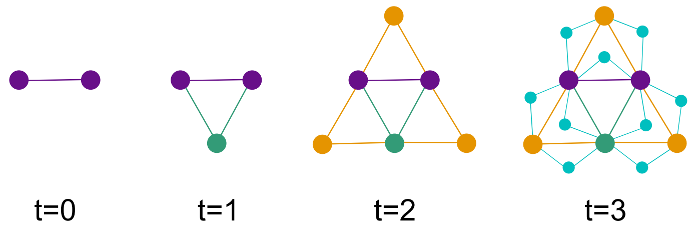


FIG. 7. Construction of the $(1, 2)$-*flowers* at steps $t = 0, 1, 2, 3$.

Such a procedure generates different types of graphs. Hence, $(> 1, v)$-*flowers* are known to exhibit finite Hausdorff dimension, $d_H$, while $(1, v)$-*flowers* have been called transfinite fractals (transfractals) and hold strong small-world properties with infinite Hausdorff dimension. In particular, all the derivations of $d_H$ are based on rescaling analyses of the diameter of the graph $L$ (e.g., $N(L + \ell) = e^{\ell \tilde{d}_f} N(L)$, $N$ number of nodes) instead of a multiplicative one (e.g., $N(bL) = be^{d_f} N(L)$). However, we note that the general spectral dimension of both types of networks is $d_s = \log(u + v)/\log(uv)$, corresponding to the analysis of the Fiedler eigenvalue in Figure 9. Note also that, as expected for usual deterministic and recursively growing fractals [6], periodic oscillations are observed and detected by the specific heat as exemplified in Fig. 8.

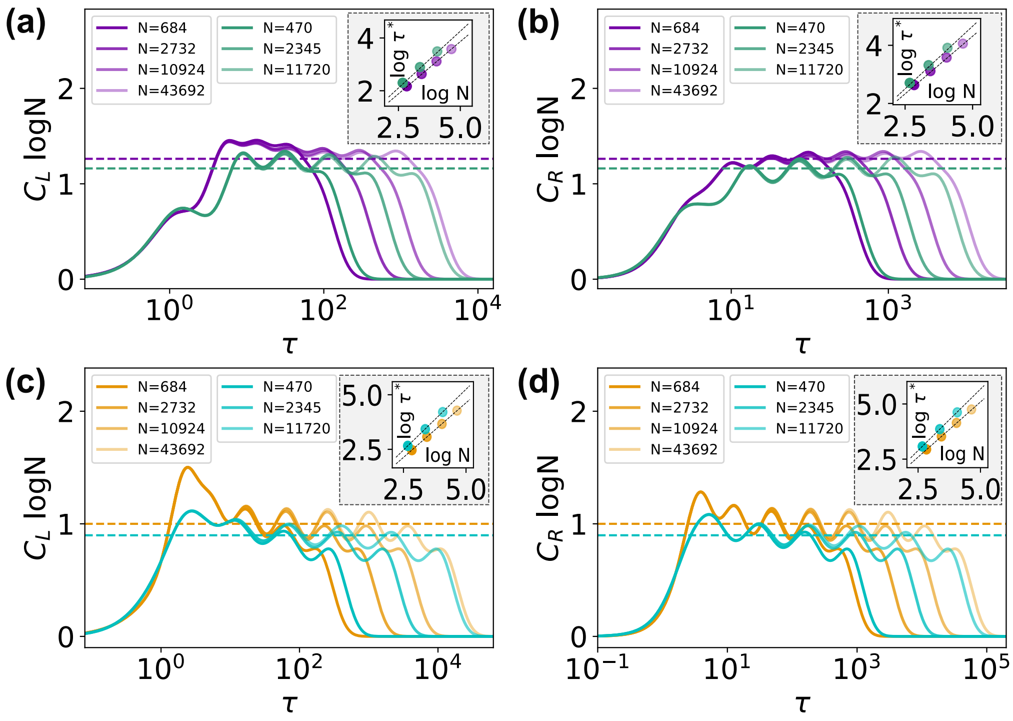


FIG. 8. **(u,v)-flowers.** Specific heat versus diffusion time $\tau$ for different system sizes (see legend) for $(1,3)$-*flowers* (purple solid line) and $(1,4)$-*flowers* (green solid line) by using **(a)** $\hat{L}$, and **(b)** $\hat{L}_{RW}$, and $(2,2)$-*flowers* (orange solid line) and $(2,3)$-*flowers* (cyan solid line) by using **(c)** $\hat{L}$ and **(d)** $\hat{L}_{RW}$. The colored horizontal dashed lines display the theoretical value of $d_S/2$, and the black dashed lines in the sub-panels show the theoretical scaling of $C_F$ as suggested in the main text.

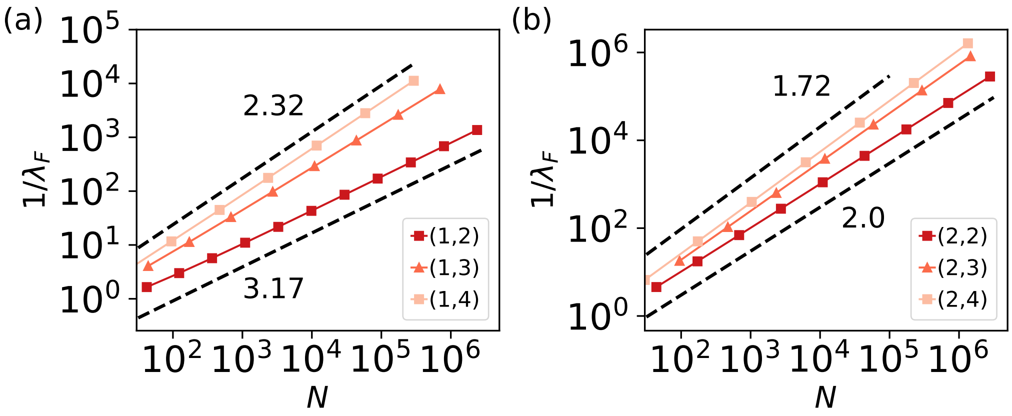


FIG. 9. **Spectral dimension for (u,v) networks.** Scaling of the inverse of the Fiedler eigenvalue versus system size for different $(u, v)$ networks and different values of $v$ (see legend) by using the Laplacian $\hat{L}$ for (a) $u = 1$, (b) $u = 2$. In all cases, these networks are scale-invariant with variable spectral dimensions.

## 8. KIM AND HOLME NETWORKS

The analysis of standard BA networks with an extended mechanism to include a 'triad formation step' is particularly interesting to explore possible mechanisms to generate self-similar networks with $d_S > 2$ [7]. Therefore, the generation mechanism proposed by Kim and Holme (KH) works by adding a new step to the preferential attachment rule as follows:

(i) A vertex, v, with m edges is added at each time step. The growth time $t$ is identified as the number of time steps.

(ii) Preferential attachment rule (PA): Each edge of $v$ is then linked to an already existing vertex with probability proportional to its degree, namely, $P_i = \frac{\kappa_i}{\sum_j \kappa_j}$.

(iii) Triad formation (TF): After each PA step in which a new vertex v is added and some edge $(u, v)$ is added, a triangle is closed with probability $p$ by choosing a neighbor of $u$, $u2$ and adding the edge $(v, u2)$.

Here, we investigate whether KH networks show any power-law scaling of the Fielder eigenvalue for different values of $m$ and $p$. Let us highlight that the case with $m = 1$ is rather trivial because it is impossible to close any triangle. Consequently, this latter mechanism will produce results identical to those of a simple BA network with $m = 1$. The results of the different types of KH networks (that is, the values of $m$) for different TF probabilities are reported in Figure 10, making it evident that only KH networks with $p = 1$ generate scale-invariant structures, as shown in the main text. In particular, the spectral dimension of the generated networks ranges from $d_S = 2.57(1)$ and $d_S = 3.65(1)$ for large values of $m$, as shown in Figure 11(b). Figure11(a) and Figure11(c) shows a specific example of these networks with $m = 2$ and $m = 3$.

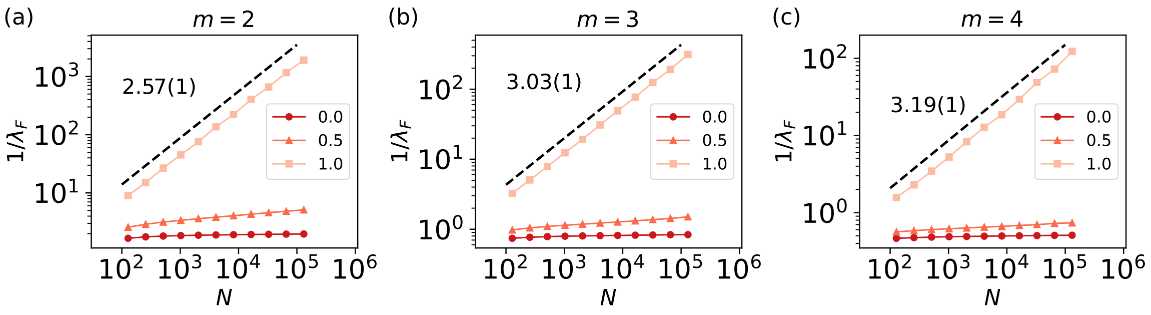


FIG. 10. **KH scale-invariant networks.** Scaling of the inverse of the Fiedler eigenvalue versus system size for different KH networks and different values of $p$ (see legend) by using the Laplacian $\hat{L}$ for (a) $m = 2$, (b) $m = 3$, and (c) $m = 4$. In all cases, only the case with $p = 1$ is truly scale-invariant with variable spectral dimension.

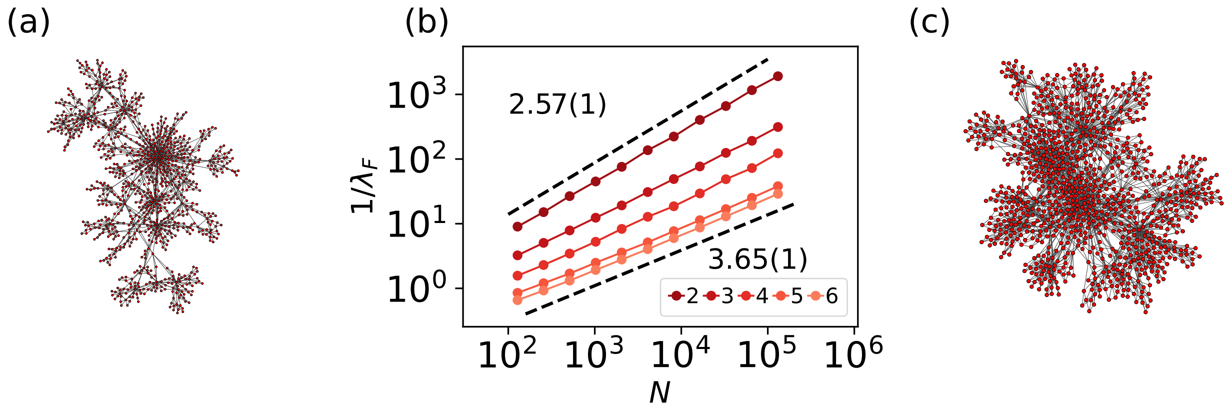


FIG. 11. **KH networks.** (a) KH network with $m = 2$, $p = 1$ and $N = 1000$. (b) Scaling of the inverse of the Fiedler eigenvalue versus system size for different KH networks with $p = 1$ and varying $m$ (see legend). The spectral dimension of the networks range from $d_S = 2.57(1)$ to $d_S = 3.65(1)$ for large values of $m$. (b) KH network with $m = 3$, $p = 1$ and $N = 1000$.

## 9. DYSON NETWORK

The Dyson graph is a weighted, fully connected, and deterministic graph. It was originally introduced by Dyson [8] to determine the occurrence of a phase transition in a one-dimensional chain with long-range interactions.

In the initial step, the network consists of a dimer with a weight link $J(d = 1, t = 1, \sigma) = 4^{-\sigma}$. Here, $t$ is the iteration step, which is an integer $\geq 1$, such that the initial configuration of the dimer is called $G(1)$. $d$ is the distance between two nodes and corresponds to the iteration step where they have been connected. In the next step, the graph is duplicated and all missing links are filled with a weight connection $J(d = 2, t = 2, \sigma) = 4^{-2\sigma}$. The same quantity is added to the weight of the old links, which now reads as $J(d = 1, t = 2, \sigma) = J(d = 1, t = 1, \sigma) + 4^{-2\sigma}$. Generalizing we get $J(d, t-1, \sigma) \to J(d, t, \sigma) = J(d, t-1, \sigma) + J(t, t, \sigma)$. Then it follows that each node will hold a unique degree $w \equiv w_i = \sum_{i \neq j} J_{ij} = \sum_{d=1}^{T} 2^{d-1} J(d, T, \sigma)$, where $J(d, T, \sigma) = \sum_{l=d}^{T} J(l, t, \sigma)$. Thus, the parameter $\sigma$ can be adjusted to modulate the decay of the interaction strength. In particular, its value affects the resulting spectral dimension that can be written as $d_S = 2/(2\sigma - 1)$. Finally, we have to add that $\sigma$ is bounded as follows: $1/2 < \sigma \leq 1$. The lower bound ensures the finite value of $w$. The upper bound does not let the inverse of the spectral gap grow faster than the system size.

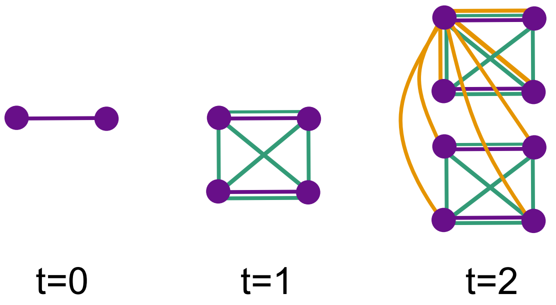


FIG. 12. Construction of Dyson graph at steps $t = 0, 1, 2$. For the sake of clarity, at step $t = 2$, only the new links involving the first node have been reported. The rest of the nodes will follow the same building rule.

Figure 13 shows the constant specific heat for different Dyson graphs with $\sigma = 0.85$ and $\sigma = 0.95$ and different system sizes. Note that these graphs can generate networks of arbitrary spectral dimension.

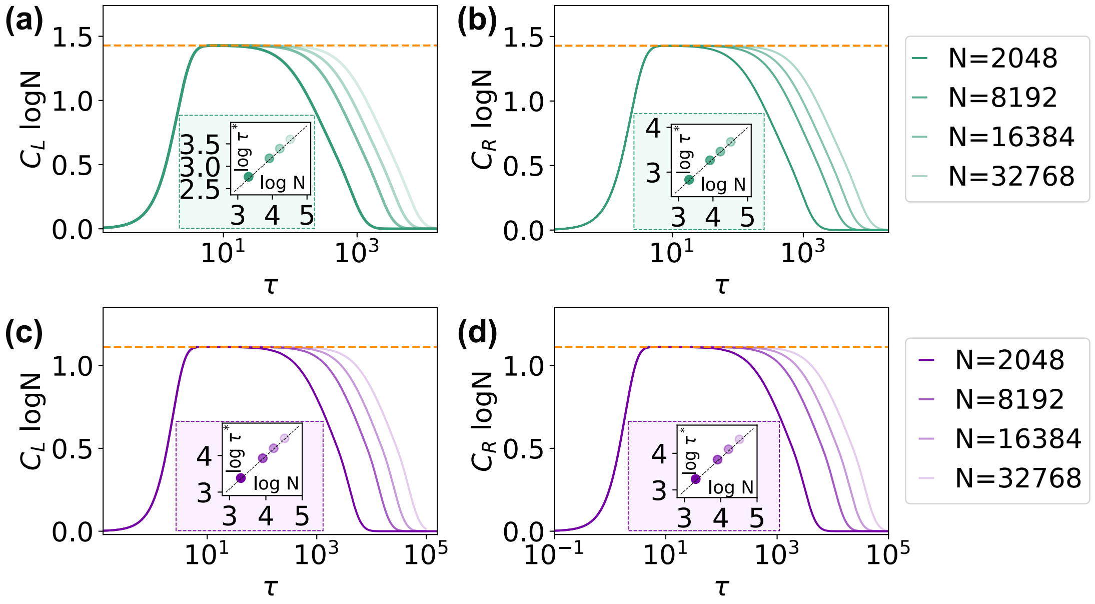


FIG. 13. **Dyson graphs.** Specific heat versus diffusion time $\tau$ for different system sizes (see legend) for $\sigma = 0.85$ using **(a)** $\hat{L}$ and **(b)** $\hat{L}_{RW}$, and $\sigma = 0.95$ using **(c)** $\hat{L}$ and **(d)** $\hat{L}_{RW}$. The colored horizontal dashed lines display the theoretical value of $d_S/2$, and the black dashed lines in the sub-panels show the theoretical scaling of $C_F$ as suggested in the main text.

## 10. HMN NETWORKS

We have also analyzed the synthetic hierarchical networks originally developed in [9]. These networks, called Hierarchic Modular Networks (HMNs), have been specifically generated to closely resemble the structure of real brain networks. In particular, HMN consists of N nodes or neurons and L links or synapses, organized into hierarchical levels for easy analysis. The HMN model that we exemplify here uses a bottom-to-top approach. First, we construct local fully connected modules and group them recursively by establishing new inter-modular links in a deterministic manner with a level-dependent number of connections (HMN).

Hence, the growing algorithm works as follows, as detailed in [9]:

(i) At each hierarchical level $l = 1, 2, ..., s$, different pairs of blocks are selected, each with size $2^{i-1}M_0$. All possible undirected $4^{i-1}M_0^2$ connections between the two blocks are evaluated and established to avoid repetitions.

(ii) The number of connections between blocks at each level is set a priori at a constant value $\alpha$.

(iii) This method is stochastic in assigning connections, although the number of them (as well as the degree of the network) is fixed deterministically, being,

$$\langle \kappa \rangle = M_0 - 1 + \frac{2\alpha}{M_0}(1 - 2^{-s}).$$

Figure 14 shows the eigenvalue probability distribution for HMNs with $M_0 = 2$ and different values of $\alpha$. Note the power-law scaling for small values of $\lambda$, where the number of oscillations increases with the number of hierarchical levels, $s$. Figure 15 shows the inverse of the Fielder eigenvalue for different classes of HMN networks using fully connected cliques of size $M_0 = 2$, $M_0 = 3$, and $M_0 = 4$ as basal blocks. In particular, we observe that the spectral dimension of these specific networks continuously varies over the interval $d_S \in (1.25, 2)$.

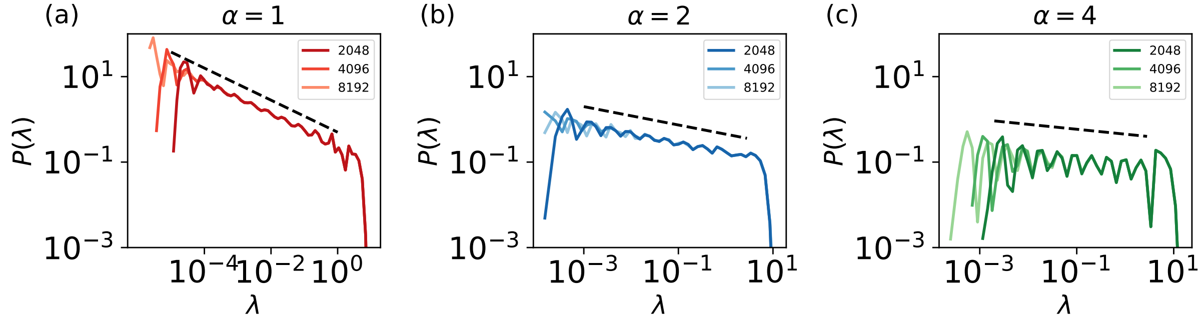


FIG. 14. **HMN eigenvalues.** Eigenvalue probability distribution for HMN networks with $M_0 = 2$ and different system sizes (see legend) by using the Laplacian $\hat{L}$ for (a) $\alpha = 1$, (b) $\alpha = 2$, and (c) $\alpha = 4$. All curves have been averaged over $10^3$ independent realizations. Dashed lines represent the scaling $P(\lambda) \propto \lambda^{d_S/2-1}$.

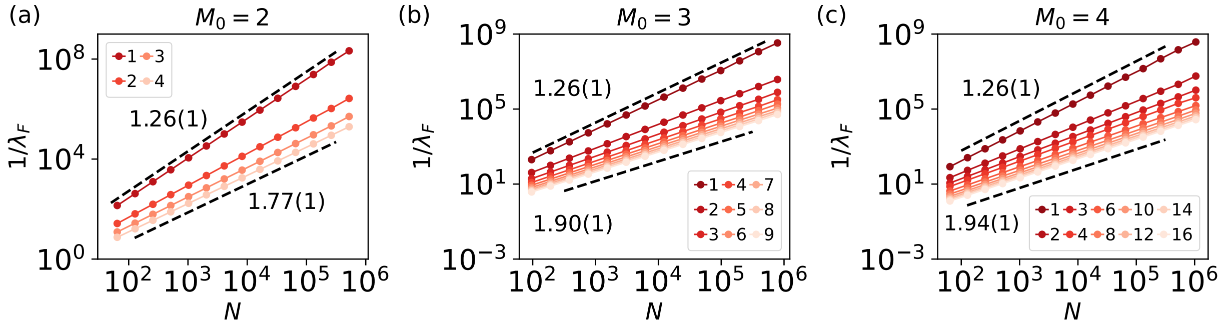


FIG. 15. **HMN spectral dimension.** Scaling of the inverse of the Fiedler eigenvalue versus system size for different HMN networks and different values of $\alpha$ (see legend) by using the Laplacian $\hat{L}$ for (a) $M_0 = 2$, (b) $M_0 = 3$, and (c) $M_0 = 4$. In all cases, HMN are scale-invariant networks with variable spectral dimensions.

Figure 16 shows the constant specific heat for different HMN networks for $M_0 = 2$ and different values of $\alpha$. Note that all networks present a constant specific heat, either for $C_L$ and $C_R$ with the expected theoretical value of $d_S$.

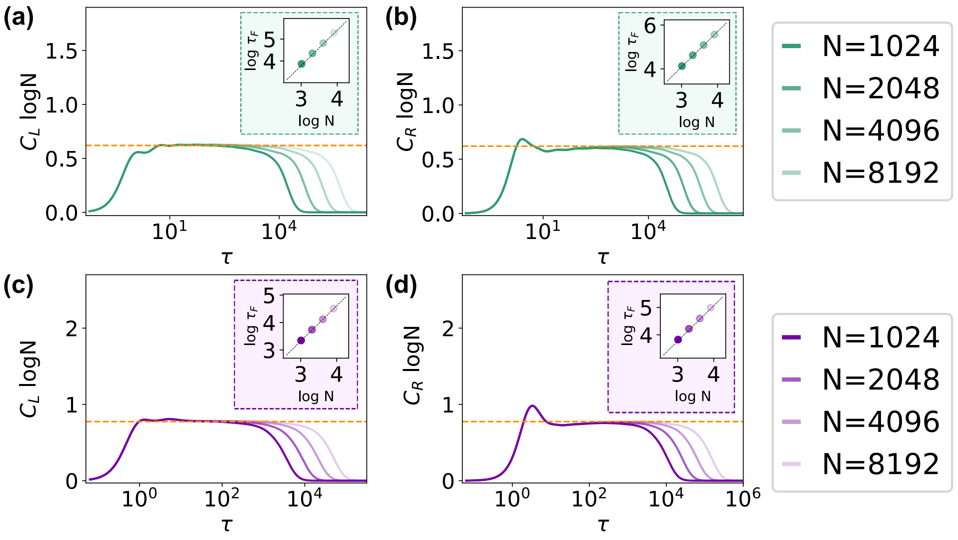


FIG. 16. **HMN graphs.** Specific heat versus diffusion time $\tau$ for $M_0 = 2$ and $\alpha = 1$ using **(a)** $\hat{L}$ and **(b)** $\hat{L}_{RW}$, and $M_0 = 2$ and $\alpha = 2$ using **(c)** $\hat{L}$ and **(d)** $\hat{L}_{RW}$. The colored horizontal dashed lines display the plateau level, and the black dashed lines in the sub-panels show the theoretical scaling of $C_F$, as suggested in the main text. All curves have been averaged over $10^3$ network realizations.

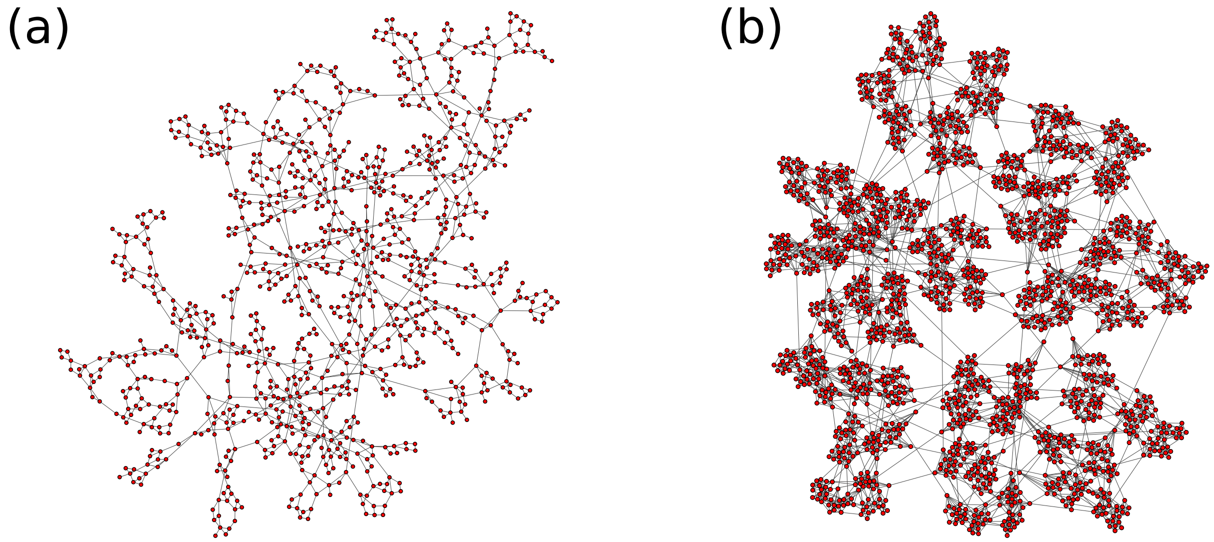


FIG. 17. **HMN networks.** (a) HMN network with $M_0 = 2$, $\alpha = 2$ and $s = 9$ hierarchical levels. (b) HMN network with $M_0 = 4$, $\alpha = 10$ and $s = 9$ hierarchical levels.

## 11. HUMAN CONNECTOME NETWORK

We have also analyzed the intrinsic structure of the Human Connectome Network (HC), a reconstruction of structural brain networks composed of hundreds of neural regions and thousands of white-matter fiber interconnections. This network consists of 998 nodes, each representing a mesoscopic population of neurons whose mutual connections are encoded by a symmetric weighted connectivity matrix. In particular, it is well-known that the HC is organized in modules and structured in a hierarchical fashion across many scales.

To uncover incipient scale-invariant features in HC, we have filtered the weighted HC matrix by imposing a threshold $T$ below which the links are discarded (without performing any network binarization). We emphasize that, as a function of this threshold $T$, a random tree will always emerge, forming the backbone of the giant component of every network at the percolation threshold. However, here we observe that the network exhibits a kind of plateau near $d_S \approx 2$ for $T \in (2 \cdot 10^{-2}, 5 \cdot 10^{-2})$, which is consistent with our previous results for HMN networks. Figure 18(a) shows the fraction of nodes belonging to the giant cluster ($P_\infty$) and the remaining fraction of edges regarding their initial number ($E_\infty$) when we sparsify the network. Note that at some specific value of $T \approx 6 \cdot 10^{-2}$, the resulting giant component corresponds to a random tree at the critical point of percolation. Instead, Figure 18(b) shows the resulting specific heat for the giant connected component of the sparsified network. Figure 19 shows the resulting networks for the different values of T analyzed in Figure18(b).

Finally, to check whether the HC network actually exhibits scale-invariant properties, we performed iterative coarse-graining of the network using the LRG [10] and monitored the scaling of the Fiedler vector for different system sizes. We used the density matrix $\rho(\tau)$ to define a network dendrogram as explicitly described in [10, 11]. Hence, by applying Ward's method to analyze the HC network clusters, it is possible to cut the dendrogram at different heights to generate reduced networks of smaller sizes, as shown in the main text.

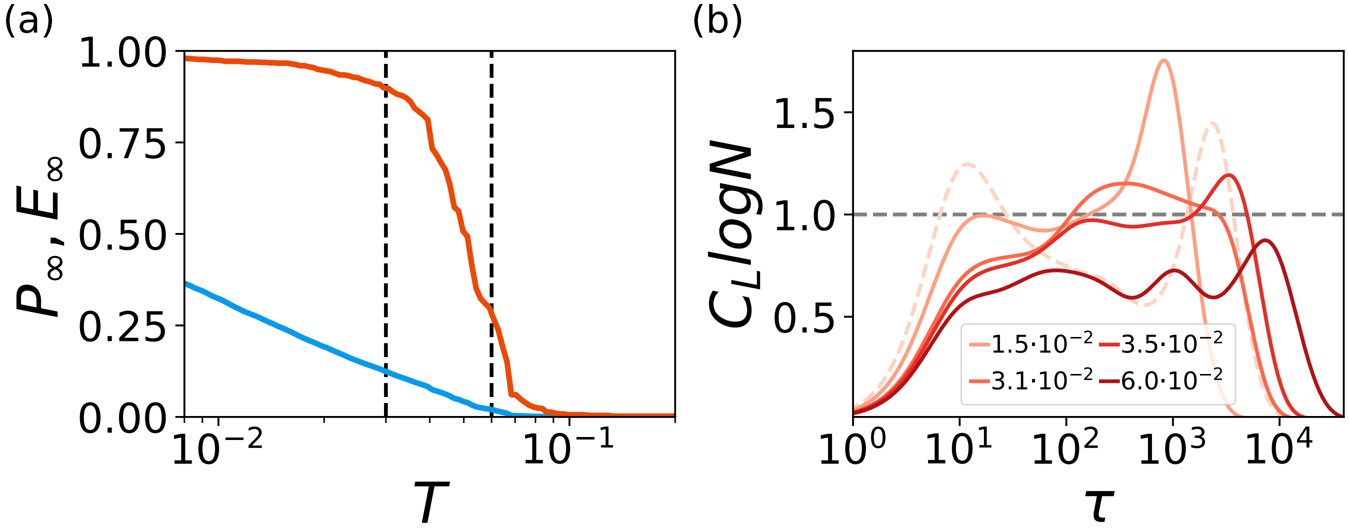


FIG. 18. (a) Giant cluster size ($P_\infty$) and fraction of edges regarding the total original ones ($E_\infty$) versus sparsification threshold $T$. The network shows a usual percolation phase transition for $T \approx 0.6$, while a non-trivial network structure still emerges with a non-vanishing giant component for threshold values $T \in (2 \cdot 10^{-2}, 5 \cdot 10^{-2})$. (b) Specific heat versus diffusion time for different values of $T$ (see legend). Values of T within $(2 \cdot 10^{-2}, 5 \cdot 10^{-2})$ are compatible with a spectral dimension $d_S \approx 1.9(1)$, while for $T \approx 0.6$ a random tree with spectral dimension $d_S = 4/3$ emerges, as expected for any percolation phase transition.

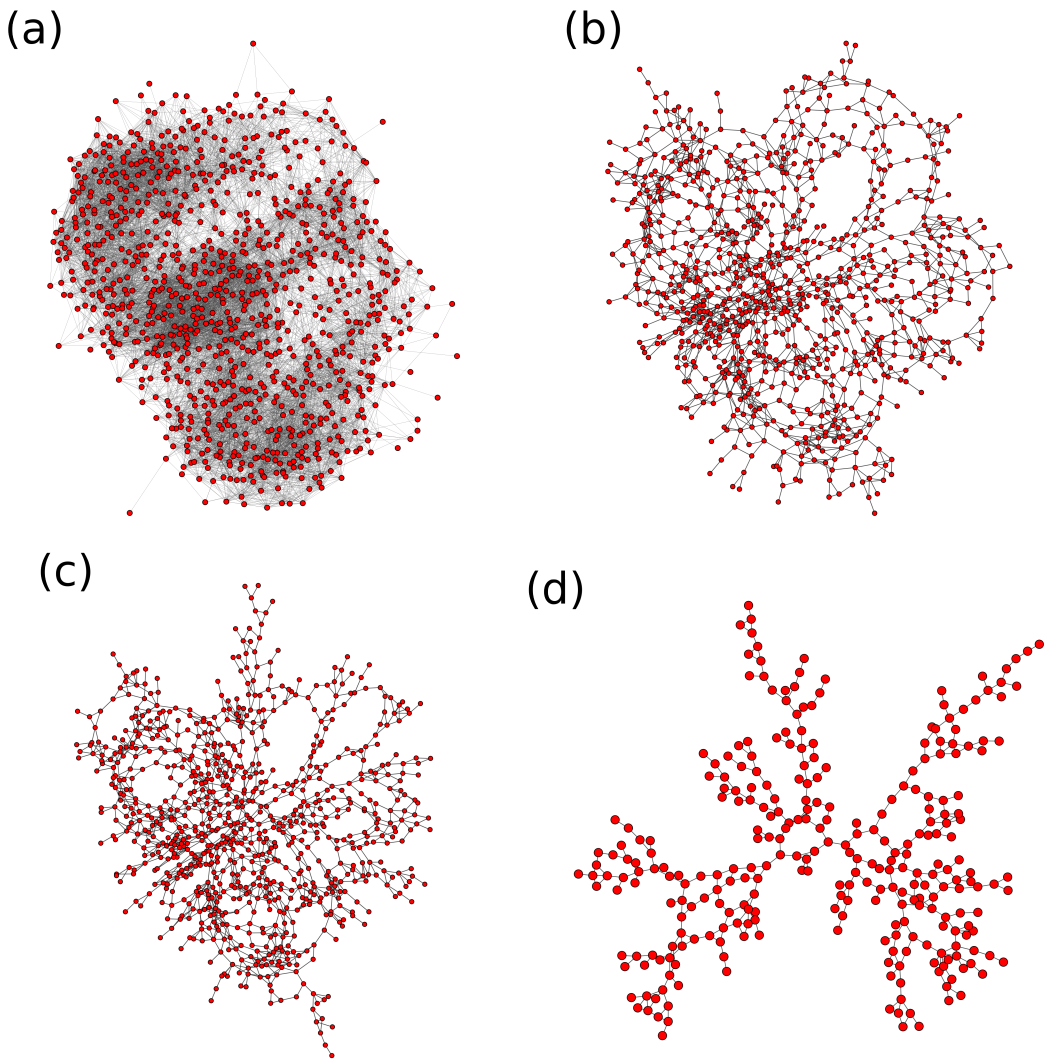


FIG. 19. Human Connectome network Giant cluster network for different threshold values. (a) $T = 10^{-3}$, (b) $T = 3 \cdot 10^{-2}$, (c) $T = 3.5 \cdot 10^{-2}$, and (d) $T = 6 \cdot 10^{-2}$. Note that, for the last case, the giant cluster of the network corresponds to a random tree as expected for a usual percolation phase transition.

## REFERENCES


[1] K. C. Das, The laplacian spectrum, Comput. Math. Appl. **48**, 715 (2004).

[2] S. N. Dorogovtsev and J. F. Mendes, *The nature of complex networks* (Oxford University Press, Oxford, 2022).

[3] R. Burioni and D. Cassi, Random walks on graphs: ideas, techniques and results, J. Phys. A **38**, R45 (2005).

[4] A. Erzan and A. Tuncer, Explicit construction of the eigenvectors and eigenvalues of the graph laplacian on the cayley tree, Linear Algebra Its Appl. **586**, 111–129 (2020).

[5] H. D. Rozenfeld, S. Havlin, and D. Ben-Avraham, Fractal and transfractal recursive scale-free nets, New J. Phys. **9**, 175 (2007).

[6] T. Vicsek, M. Shlesinger, and M. Matsushita, *Fractals in Natural Sciences* (World Scientific, Singapore, 1994).

[7] P. Holme and B. J. Kim, Growing scale-free networks with tunable clustering, Phys. Rev. E **65**, 026107 (2002).

[8] F. J. Dyson, Existence of a phase-transition in a one-dimensional ising ferromagnet, Commun. Math. Phys. **12**, 91 (1969).

[9] P. Moretti and M. A. Muñoz, Griffiths phases and the stretching of criticality in brain networks, Nat. Comm. **4**, 2521 (2013).

[10] P. Villegas, T. Gili, G. Caldarelli, and A. Gabrielli, Laplacian renormalization group for heterogeneous networks, Nat. Phys. **19**, 445–450 (2023).

[11] P. Villegas, A. Gabrielli, A. Poggialini, and T. Gili, Multi-scale laplacian community detection in heterogeneous networks, arXiv (2023), 2301.04514.
